# Supplementary material for: Expanding the reach of quantum optimization with fermionic embeddings
Source: arXiv:2301.01778 source file (2024-08-20)
Supplement: Supplementary file 1 [file appendix_group-sync.tex]

Because the group synchronization problem is a particularly important instance of the LNCG problem, here we describe some prominent properties of this problem within our quantum formalism. Recall that in the group synchronization problem, the planted solution $g_1, \ldots, g_m \in G$ gives rise to interaction terms of the form $g_{uv} = g_u^\T g_v$. When the measurements of this interaction are noiseless, the objective matrices are simply $C_{uv} = g_{uv}$. In this appendix we demonstrate two features of the resulting Hamiltonian:~first, due to the planted nature of the problem every instance of the noiseless group synchronization Hamiltonian is unitarily equivalent to a single instance wherein all $C_{uv} = I$. Second, the Hamiltonian possesses an additional symmetry which transfers the action of left multiplication to right multiplication. In both cases, the key unitary transformations are also simple tensor products of free-fermion rotations, although their structures are different from the universal $\Orth(n)$ symmetry discussed in Sec.~\ref{}.

Although the noiseless problem is straightforward to solve classically, the difficult case of noisy measurements $C_{uv} = g_u^\T g_v + \sigma W_{uv}$ can be studied by treating the additive term as a small perturbation. For instance, a typical noise model treats the entries of $W_{uv}$ as normally distributed and $\sigma > 0$ a noise-strength parameter. Therefore understanding the properties of the noiseless instance should be useful for future studies of this problem.

\subsection{Reduction to the $C_{uv} = I$ case}

Because each objective matrix takes the form $C_{uv} = g_u g_v^\T$, a simple rewriting of the Hamiltonian allows us to decouple the interaction terms:
\begin{equation}
\begin{split}
    H &= \sum_{(u, v) \in E} \sum_{i,j \in [n]} \sum_{\ell \in [n]} [g_u]_{i\ell} [g_v]_{j\ell} \sum_{k \in [n]} P_{ik}^{(u)} \otimes P_{jk}^{(v)}\\
    &= \sum_{(u, v) \in E} \sum_{k, \ell \in [n]} \i \l( \sum_{i \in [n]} [g_u]_{i\ell} \widetilde{\gamma}_i^{(u)} \r) \gamma_k^{(u)} \otimes \i \l( \sum_{j \in [n]} [g_v]_{j\ell} \widetilde{\gamma}_j^{(v)} \r) \gamma_k^{(v)}.
\end{split}
\end{equation}
Each $\gamma$-type Majorana operator is therefore simply being rotated by a local free-fermion transformation,
\begin{equation}
    \sum_{i \in [n]} [g_u]_{i\ell} \widetilde{\gamma}_i^{(u)} = \mathcal{U}(g_u)^\dagger \widetilde{\gamma}_\ell^{(u)} \mathcal{U}(g_u).
\end{equation}
Then, defining the unitary operator $\mathcal{V} = \bigotimes_{v \in V} \mathcal{U}(g_v)$ which acts on the entire graph, we see that the Hamiltonian can expressed as
\begin{equation}
    H = \mathcal{V}^\dagger \l( \sum_{(u, v) \in E} \sum_{k, \ell \in [n]} P_{\ell k}^{(u)} \otimes P_{\ell k}^{(v)} \r) \mathcal{V},
\end{equation}
where $H' = \mathcal{V} H \mathcal{V}^\dagger$ corresponds to the LNCG Hamiltonian when all $C_{uv} = I$. Of course, knowing the unitary $\mathcal{V}$ is equivalent to having solved the original problem. Nonetheless, this similarity transformation only involves free-fermion unitaries, which are well understood, and furthermore the fact that $\mathcal{V}$ is simple tensor product across vertices implies that the entanglement structure between the local qudits is identical between $H$ and $H'$. Additionally, in this form one can write each edge term as
\begin{equation}
    H_{uv} = \l( \sum_{\ell \in [n]} \widetilde{\gamma}_\ell^{(u)} \otimes \widetilde{\gamma}_\ell^{(v)} \r) \l( \sum_{k \in [n]} \gamma_k^{(u)} \otimes \gamma_k^{(v)} \r)
\end{equation}
from which it is clear that the Hamiltonian is invariant to both $\widetilde{\mathcal{U}}(R_1)^{\otimes m}$ and $\mathcal{U}(R_2)^{\otimes m}$ for all $R_1, R_2 \in \Orth(n)$.

\subsection{Hamiltonian symmetry}
